# Supplementary material for: Graph Contrastive Learning for Anomaly Detection
Source: arXiv:2108.07516 source file (2022-08-29)
Supplement: Supplementary file 1 [file appendix.tex]

\section{Implementation Details}
The detailed hyper-parameters are listed in Table~\ref{tbl:hyper}.

\subsection{Running Environment}
We implement the model by Python 3.6.8, PyTorch 1.7.0, and conduct the experiments on an Enterprise Linux Server with 40 Intel(R) Xeon(R) CPU cores (E5-2640 v4 @ 2.40 GHz and 252G memory), and a single NVIDIA Tesla v100 with 32 GB memory size.

\subsection{Evaluation of \model}

\vpara{Training and Testing settings.} For the dataset of AMiner and MAG, we use [CLS] + title + keywords [SEP] as the BERT input to get the paper embedding with dimensions of 768. The maximal length of the input tokens is set as 64. Then,  we select about 70\% researchers' graphs as the training data and use the remaining ones as the test data, which results in 675 graphs for training and 429 graphs for testing in AMiner, 1,675 graphs for training and 423 graphs for testing in MAS respectively. 

For the dataset of Alpha and Yelp, we choose about 75\% labeled nodes from the single graph as the training data and the remaining ones are used as the test data, which results in 177 nodes for training and 60 nodes for testing in Alpha, and 36,763 for training and 9,191 for testing in Yelp.

\vpara{Implementation of baselines.}
For a fair comparison, the training and test settings of all the baselines are the same as \model. The implemental details are defined as:

\begin{itemize}[leftmargin=*]
	
	\item
	\textbf{Logistic Regression.}  We conduct eigen-decomposition on all datasets to initialize node embeddings with top 64 eigenvectors.  Then we apply logistic regression to classify nodes. 
	
	\item
	\textbf{GCN~\cite{kipf2016semi}, GAT~\cite{velivckovic2017graph}, GraphSAGE~\cite{Graphsage}, and GIN~\cite{xu2018powerful}.} We leverage the implementations provided by Pytorch Geometric\footnote{https://github.com/rusty1s/pytorch\_geometric}, and set the number of convolutional layers as 2 for all general GNNs. 
 	
	\item
	\textbf{GeniePath~\cite{liu2019geniepath}, GraphConsis~\cite{liu2020alleviating}, and CARE-GNN~\cite{dou2020enhancing}.} We download the authors' official source codes and keep all the training settings as the same. The data format is transformed appropriately to fit their settings.

	\textit{GeniePath.} https://github.com/shawnwang-tech/GeniePath-pytorch
	
	\textit{GraphConsis.} https://github.com/YingtongDou/CARE-GNN
	
	\textit{CARE-GNN.} https://github.com/safe-graph/DGFraud

\end{itemize}

\begin{table}[htbp]
	\newcolumntype{?}{!{\vrule width 1pt}}
	
	\caption{Hyper-parameters of \model. Note that the settings of fine-tuning is the same as the ones in supervised learning. $d$ is dimensions of input node embedding.}
	\centering 
	\label{tbl:hyper}
	\small
	\begin{tabular}{@{}l?l@{}}
		\toprule
		
		\multicolumn{2}{c}{\textbf{Edge Update} }  \\
		\midrule
		MLPs & $\mathbb{R}^{2d \times d}$, $\mathbb{R}^{d \times d}$\\
		$\lambda$ & 0.4 \\
		\midrule
		\multicolumn{2}{c}{\textbf{Node Update} }  \\
		\midrule
		Encoder & GIN \\
		MLPs in GIN & $\mathbb{R}^{d \times d}$, $\mathbb{R}^{d \times d}$\\
		\#Layers of node update & 1 \\
		Norm & BatchNorm1d \\
		\midrule
		\multicolumn{2}{c}{\textbf{Model framework} }  \\
		\midrule
		\#Layers of \model & 2 \\
		\midrule
		\multicolumn{2}{c}{\textbf{Training Setting} }  \\
		\midrule
		\multicolumn{2}{c}{Batch size}  \\
		\midrule
		Supervised learning on AMiner, MAS &  1 \\
		Supervised learning on Alpha, Yelp &  1 \\		
		Pre-training on AMiner, MAS &  8 \\
		Pre-training on Alpha, Yelp &  1 \\
		\midrule
		\multicolumn{2}{c}{Learning Rate}  \\
		\midrule
		Pre-training &  1e-3 \\
		Fine-tuning  &  1e-4 \\
		Temperature parameter $\tau$ in Eq\eqref{eq:loss} & 0.5 \\
		Learning rate decay & Exponential decay =0.96\\
		\midrule
		\multicolumn{2}{c}{Others }  \\
		\midrule
		Corrupt Ratio & 0.15 \\
		%Maximal token length of papers in AMiner & 208 \\
		Optimization algorithm		& Adam \\
		Pre-training epochs		& 300 \\
		Fine-tuning epochs      & 100 \\
		
		\bottomrule
	\end{tabular}
	\normalsize
\end{table}

\subsection{Evaluation of \pmodel}
\spmodel is trained on pseudo anomalies labels constructed by our proposed corrupt strategy (c.f. \secref{subsec:self}), and then fine-tuned on different percentage of training data used in \model. Finally, we test the performance of \spmodel on the same test set. 

\vpara{Pre-training settings.}
For efficient training on the 4,800 corrupt academic graphs, we set the mini-batch size as 8, i.e, including 8 graphs in each batch. We further restrict the number of nodes in each graph to 64. With the corrupt ratio of 15\%, there are 54 normal nodes and  10 normal nodes in each graph. To meet negative instances as much as possible, we adapt the pre-training settings of simCLR~\cite{chen2020simple}, a popular pre-training scheme for visual representation learning, to take all the nodes from other graphs in the same batch as the negative instances in addition to the pre-injected abnormal nodes in the concerned graph. 
Notably, different from the pre-injected abnormal nodes, the sampled negative instances from other graphs during training only impact the loss function, but are regardless of the graph convolution of the concerned graph. 

Since the number of partitioned graphs in Alpha and Yelp is much smaller than that in AMiner and MAS, we set mini-batch size as 1 on them.

\vpara{Implementation of pre-training frameworks.}
We download the authors' official source code and keep all the training settings as the same. Note that, due to the pre-training baselines we compared with are designed for characterizing the normal pattern of the graph, we do not use the corrupt strategy to corrupt the clustering sub-graphs but use the sub-graph itself as the pre-training data. For a fair comparison, all the pre-training frameworks leverage the same GNN encoder \smodel.

\textit{GAE}~\cite{kipf2016variational}. https://github.com/tkipf/gae

\textit{DGI}~\cite{velickovic2019deep}. https://github.com/PetarV-/DGI

\textit{GraphCL}~\cite{you2020graph}. https://github.com/Shen-Lab/GraphCL

\textit{GPT-GNN}~\cite{hu2020gpt}. https://github.com/acbull/GPT-GNN.

For GraphCL, we try all the graph augmentation methods defined in the paper, and select the one which achieves the best performance in the test set without fine-tuning.
